# Supplementary material for: Attention De-sparsification Matters: Inducing Diversity in Digital Pathology Representation Learning
Source: arXiv:2309.06439 source file (2023-09-12)

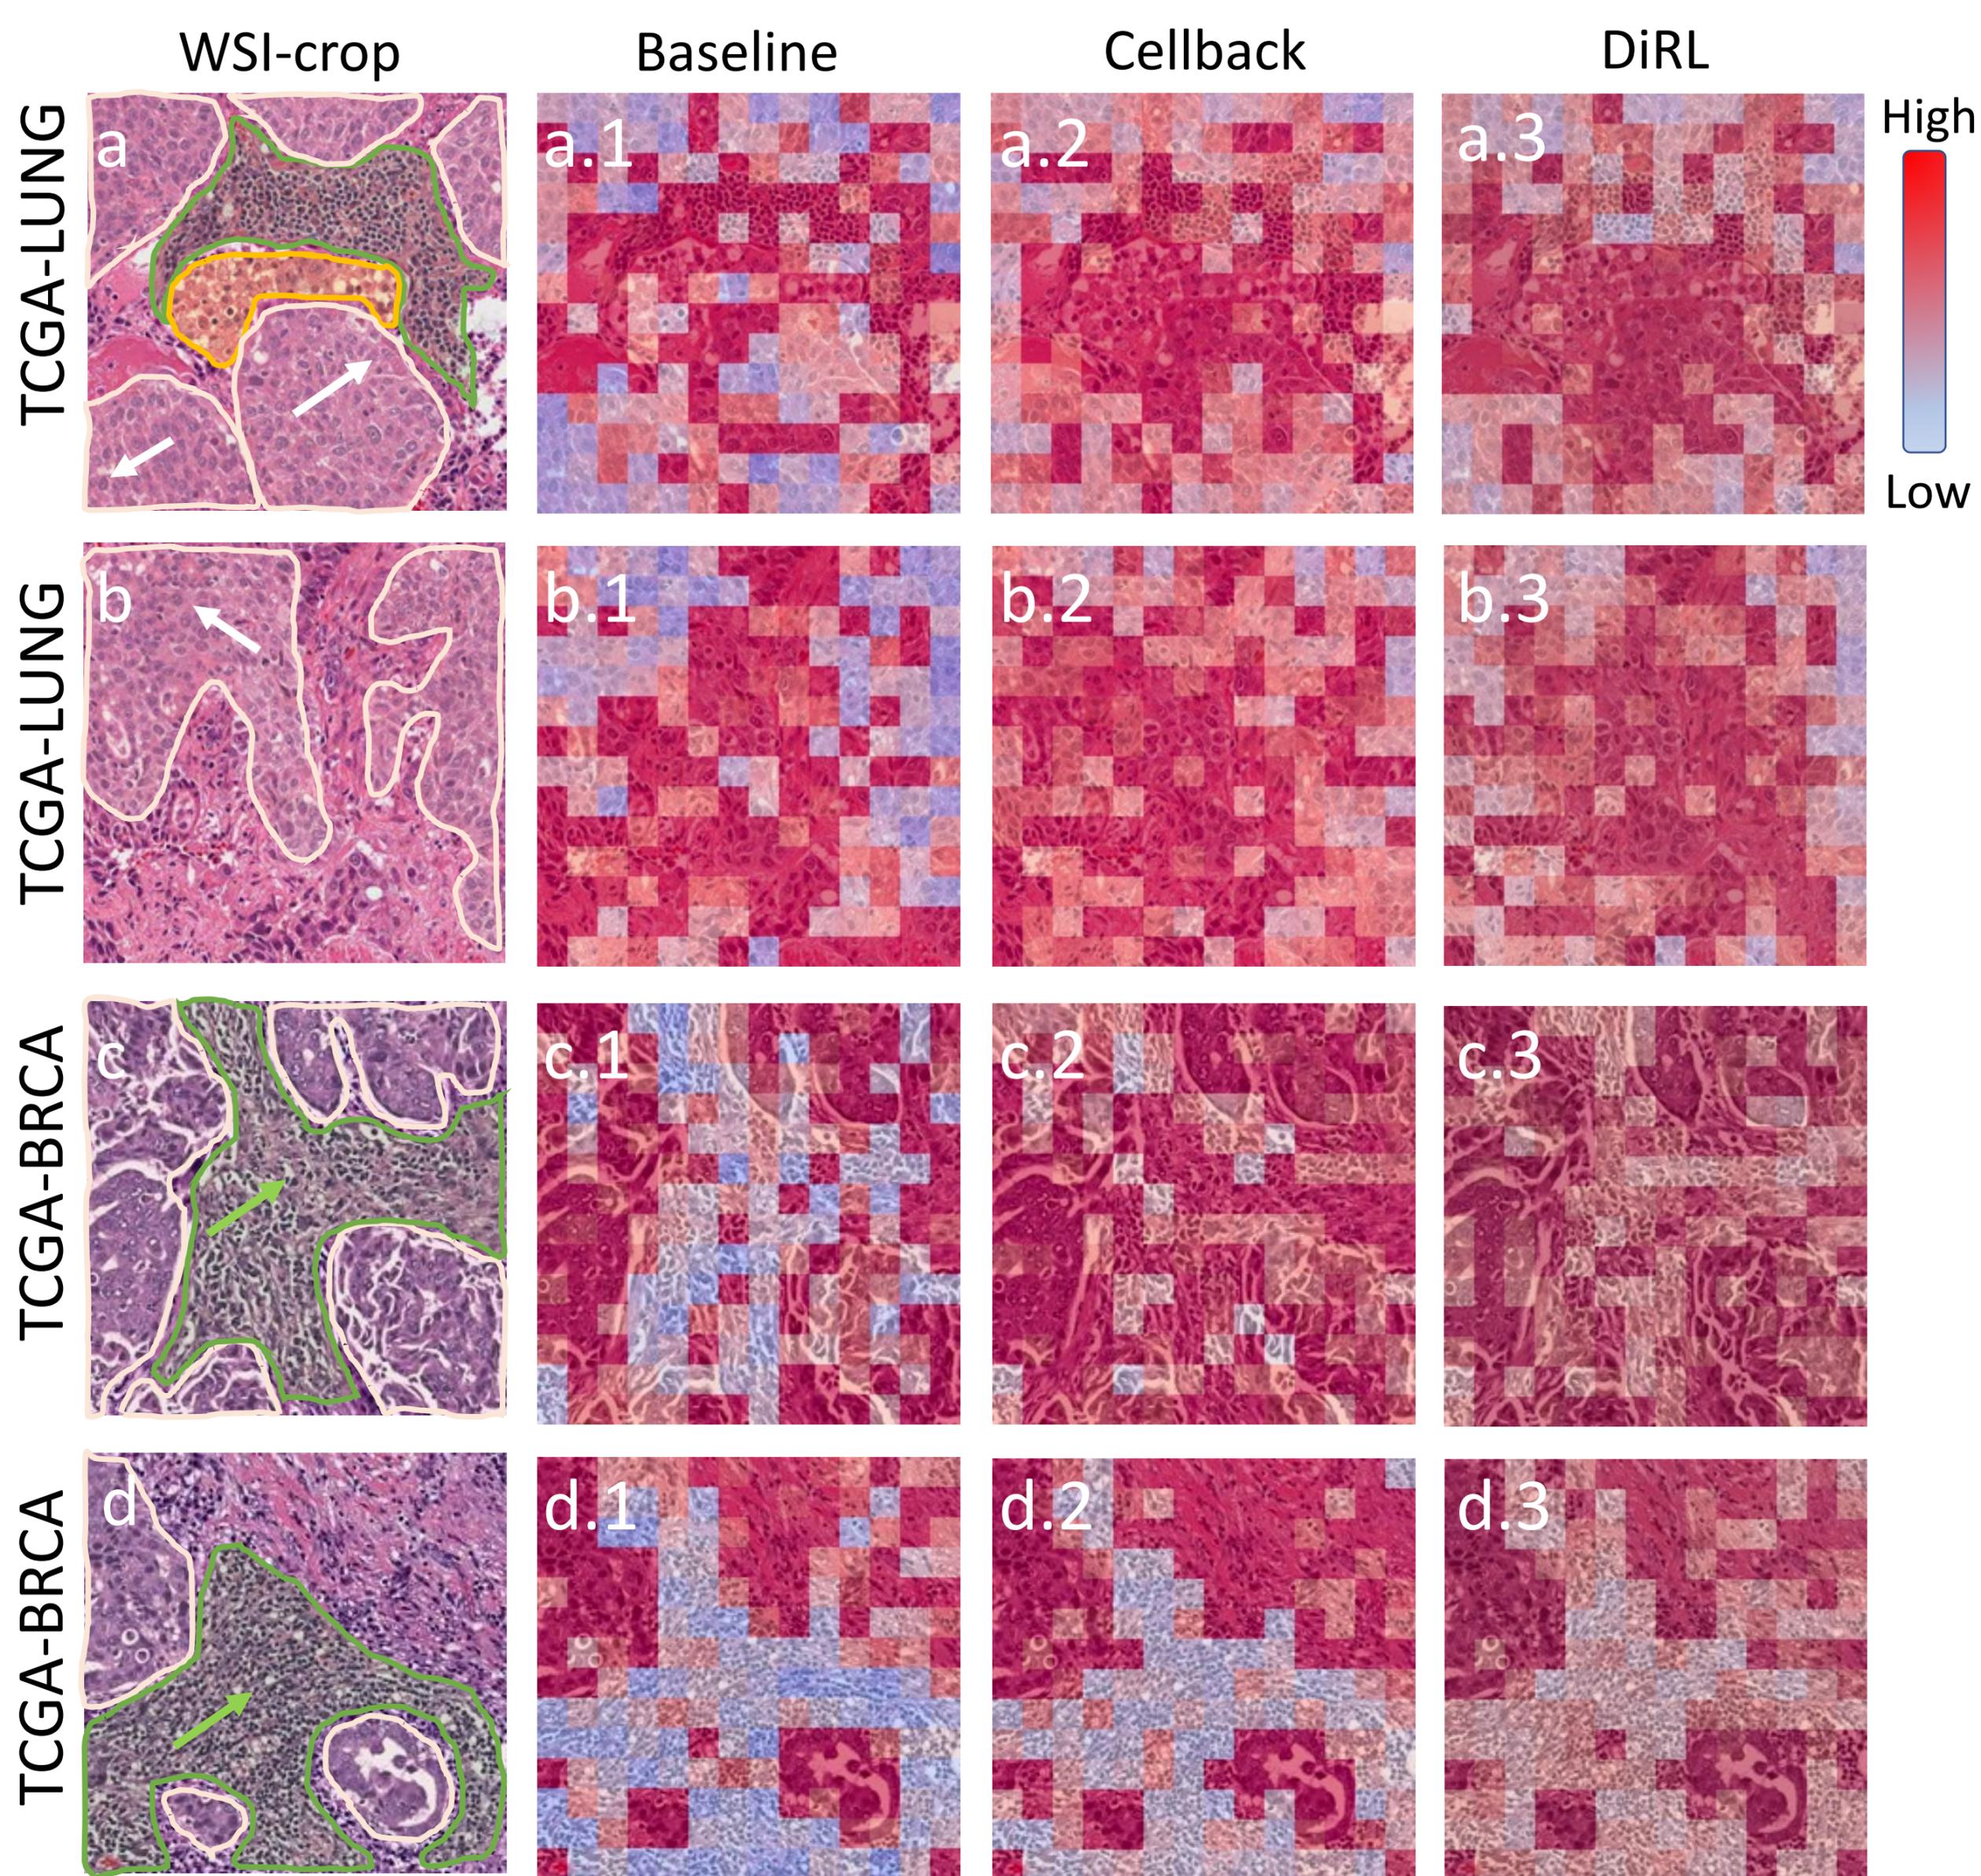

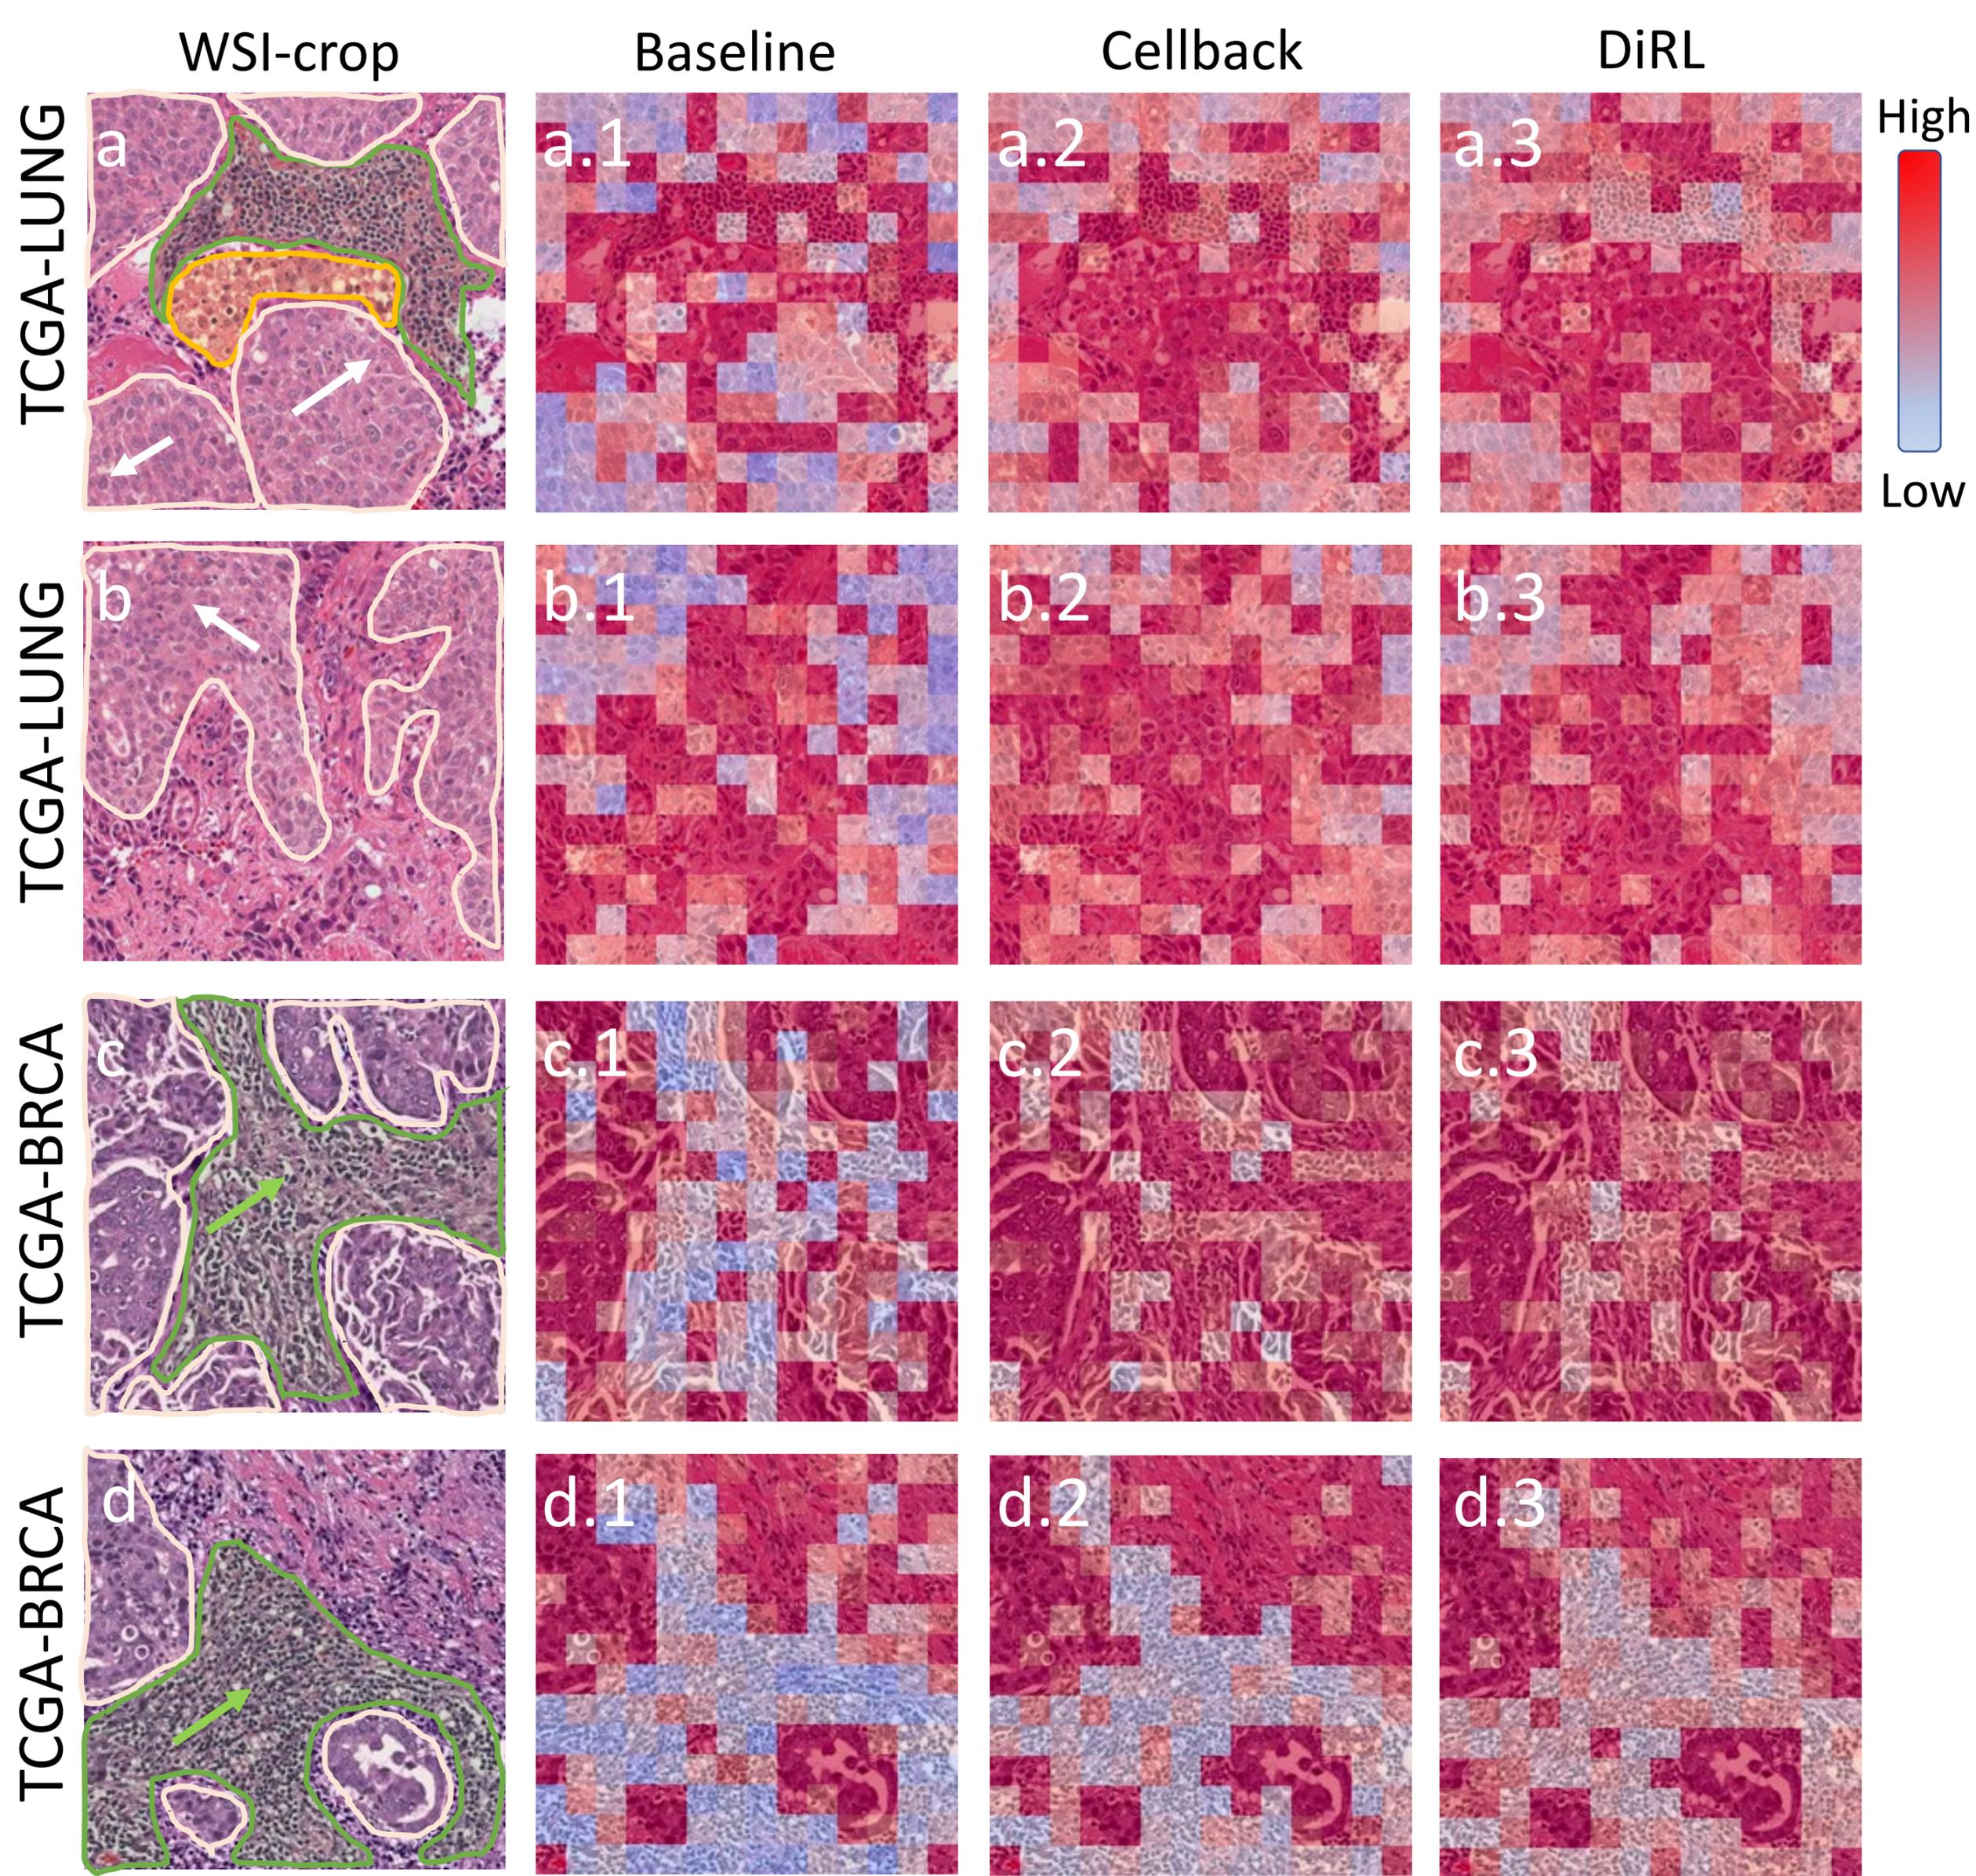

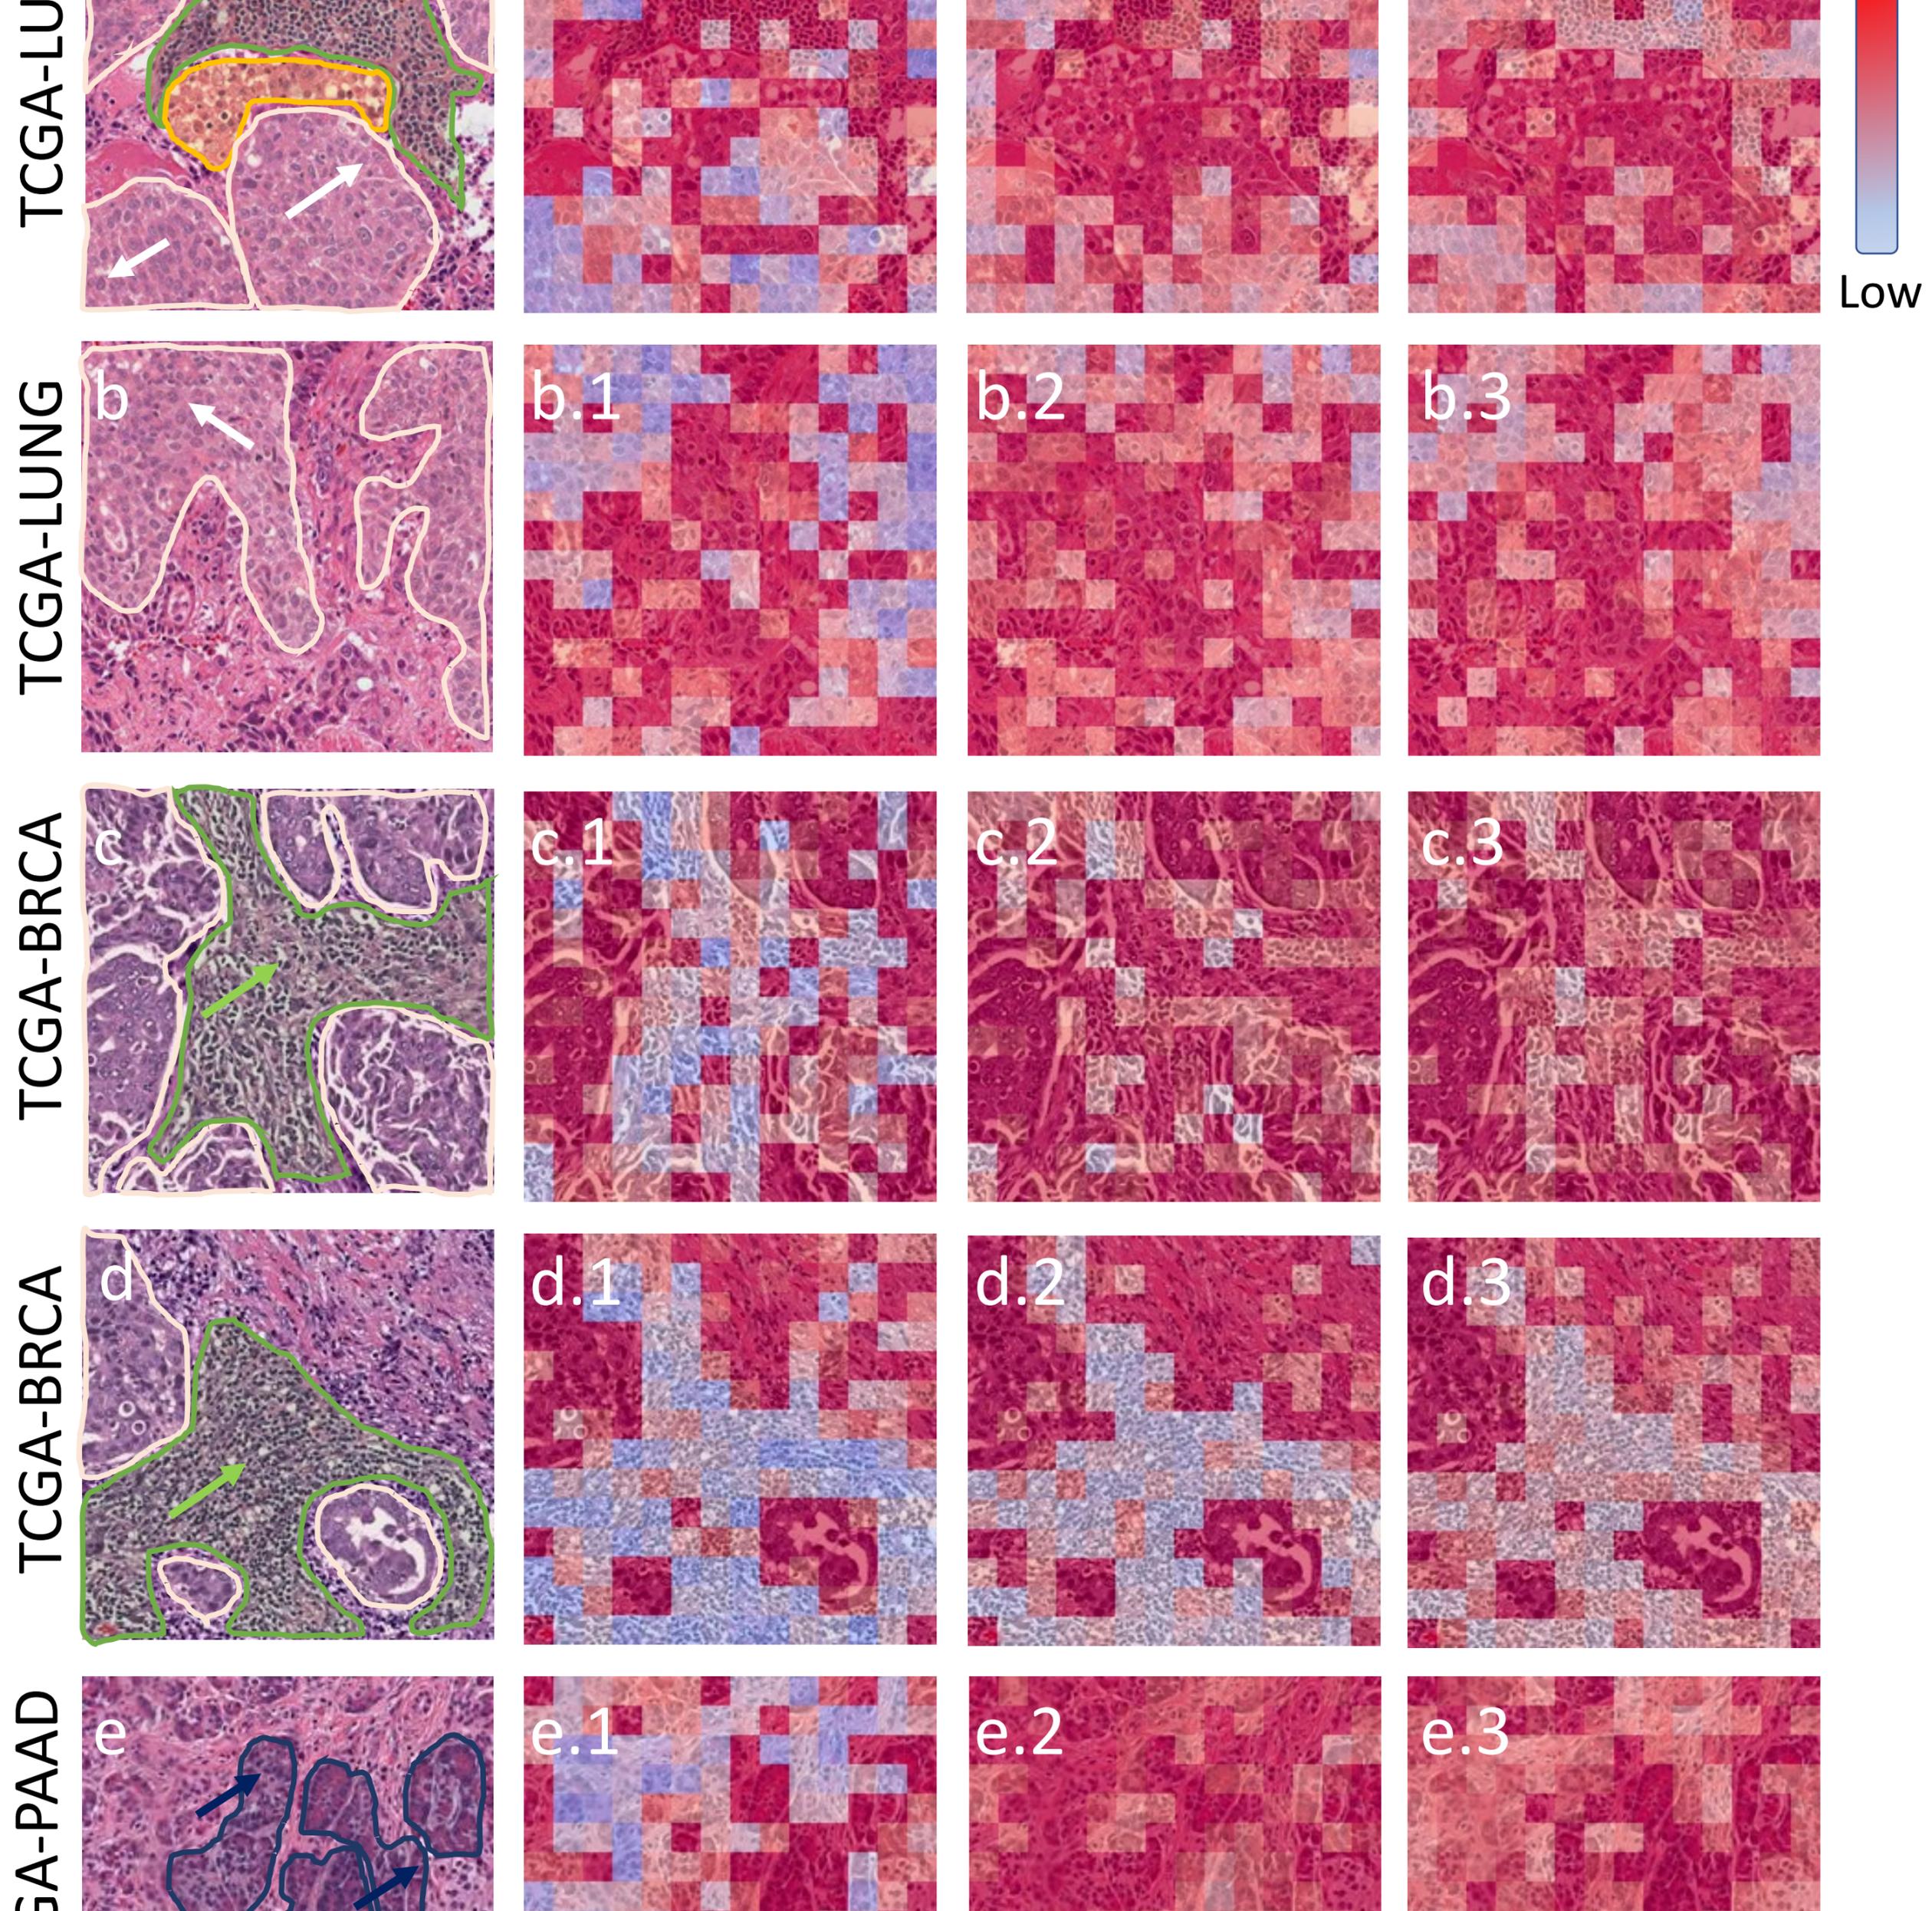

Supplement: Supplementary file 1 [file Additional_attention_visualization.pdf]
